# Supplementary material for: AgileWatts: An Energy-Efficient CPU Core Idle-State Architecture for Latency-Sensitive Server Applications
Source: arXiv:2203.02550 source file (2025-02-25)
Supplement: Supplementary file 1 [file _10_appendix.tex]

\appendix

We thank the reviewers for their valuable feedback. Below are the changes made in the paper, based on the reviewer’s feedback.

\begin{itemize}[leftmargin=5mm,nolistsep]

\item We add Fig.~\ref{fig:ppa_modeling} and footnote~\ref{footnote:leak_scal} to better explain the methodology and model used to estimate the area, power and performance of \tech. We also clarify the explanation of the modelling methodology in Sec.~\ref{sec:ppa_model_meth}.
\item We discuss \tech benefits for hierarchical AMD processors in Sec.~\ref{sec:amd_benefits}.
\item We present the impact of high snoop traffic in Sec.~\ref{sec:snoop_impact}.
\item We include Sec.~\ref{sec:DC_cost_red} to discuss data center cost savings.
\item We extend Sec.~\ref{sec:related} to include a survey for latency sensitive applications.
\item We add footnote~\ref{footnote:eval_expl} to improve the explanation of the evaluation.
\end{itemize}
